# Supplementary material for: Robust Langevin Sampling under State-Dependent Heavy-Tailed Noise with Applications to LLM Fine-Tuning
Source: arXiv:2610.12865 source file (2026-10-09)
Supplement: Supplementary file 1 [file appendix_contents.tex]

% Appendix-only contents, with hyperlink-aware entries and automatic page numbers.
% Load these definitions in the preamble; enable recording after \appendix.
\makeatletter
\newcommand{\enableappendixcontents}{%
  \let\appendix@addcontentsline\addcontentsline
  \renewcommand{\addcontentsline}[3]{%
    \appendix@addcontentsline{##1}{##2}{##3}%
    \def\appendix@extension{##1}%
    \def\appendix@toc{toc}%
    \ifx\appendix@extension\appendix@toc
      \addtocontents{apx}{%
        \protect\contentsline{##2}{##3}{\thepage}{\@currentHref}%
        \protected@file@percent
      }%
    \fi
  }%
}
\newcommand{\printappendixcontents}{%
  \pdfbookmark[0]{Appendix Table of Contents}{appendix-contents}%
  \section*{Appendix Table of Contents}%
  \begingroup
    \c@tocdepth=2\relax
    \renewcommand{\l@section}[2]{%
      \begingroup\bfseries
        \@dottedtocline{1}{0em}{1.8em}{##1}{##2}%
      \endgroup
    }%
    \renewcommand{\l@subsection}{\@dottedtocline{2}{1.8em}{2.8em}}%
    \@starttoc{apx}%
  \endgroup
}
\makeatother
